# Supplementary material for: Van der Waals functionalization of ultrahigh-Q silica microcavities for $\chi^{(2)}$-$\chi^{(3)}$ hybrid nonlinear photonics
Source: arXiv:2311.13916 ancillary file (2023-11-23)
Supplement: Supplementary file 1 [file SI_cavity_nanomaterial.pdf]

# Supplementary information to "Van der Waals functionalization of ultrahigh-Q silica microcavities for $\chi^{(2)}$-$\chi^{(3)}$ hybrid nonlinear photonics"

Shun Fujii,[1,2,*] Nan Fang,[3] Daiki Yamashita,[1,4]
Daichi Kozawa,[1,3,5] Chee Fai Fong,[3] and Yuichiro K. Kato[1,3,†]

[1]*Quantum Optoelectronics Research Team,*
*RIKEN Center for Advanced Photonics, Saitama 351-0198, Japan*
[2]*Department of Physics, Faculty of Science and Technology,*
*Keio University, Yokohama, 223-8522, Japan*
[3]*Nanoscale Quantum Photonics Laboratory,*
*RIKEN Cluster for Pioneering Research, Saitama 351-0198, Japan*
[4]*Platform Photonics Research Center,*
*National Institute of Advanced Industrial Science*
*and Technology (AIST), Ibaraki 305-8568, Japan*
[5]*Research Center for Materials, National Institute*
*for Materials Science, Ibaraki 305-0044, Japan*

[*] Corresponding author. shun.fujii@phys.keio.ac.jp
[†] Corresponding author. yuichiro.kato@riken.jp

**Supplementary Note 1: The relation between the evanescent field ratio and the cavity radius**

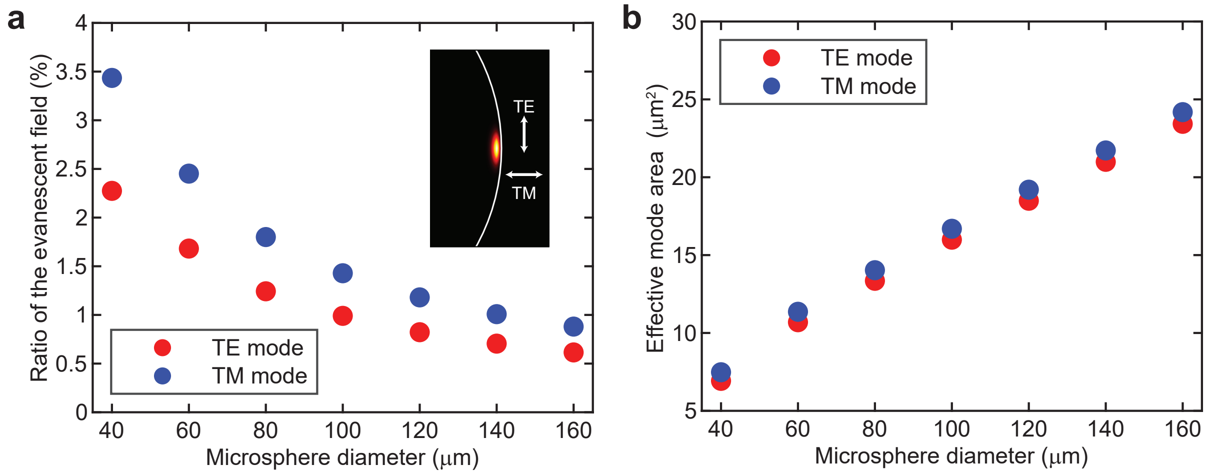


Supplementary Figure S1. The relation between mode profiles and the cavity diameter in a silica microsphere. Calculated mode ratio of the evanescent field to the total field (a) and the cavity mode area (b) as a function of the microsphere diameter for two different polarizations.

The size of a silica microsphere cavity is the key to obtaining strong light-matter interaction between the optical mode and the surface integrated transition metal dichalcogenide (TMD) flake because the ratio of the evanescent field to the total intensity is inversely proportional to the cavity size. Here, the optical mode profiles and the effective mode area are calculated by finite element method (FEM) simulation (COMSOL Multiphysics). Figure S1(a) shows the calculation result representing the ratio of the evanescent field as a function of the microsphere diameter for two different polarizations (where the TE mode is mainly along the polar direction, whereas the TM mode has two main electric-field components along the radial and azimuthal directions as shown in the inset). This result indicates that only a few percent of the mode volume interacts with the surface layer, and the TM modes exhibit a slightly higher evanescent intensity. It should be noted that the cavity mode volume is proportional to the diameter as shown in Fig. S1(b), in contrast to the evanescent ratio.

Besides, a smaller cavity has another advantage for light-matter interaction because the intracavity power circulating inside the cavity is also inversely proportional to the cavity

diameter $D$ as the intracavity power at a critical coupling condition is given by [1],

$$P_{\text{cav}} = \frac{Q f_{\text{FSR}}}{\pi f} P_{\text{in}} = \frac{Qc}{\pi^2 n D f} P_{\text{in}}, \tag{S1}$$

where $f_{\text{FSR}}$ is the free-spectral range of the cavity, $n$ is the refractive index, $f$ is the resonant frequency, and $P_{\text{in}}$ is the input power.

## Supplementary Note 2: Fabrication of 2D material-functionalized microsphere

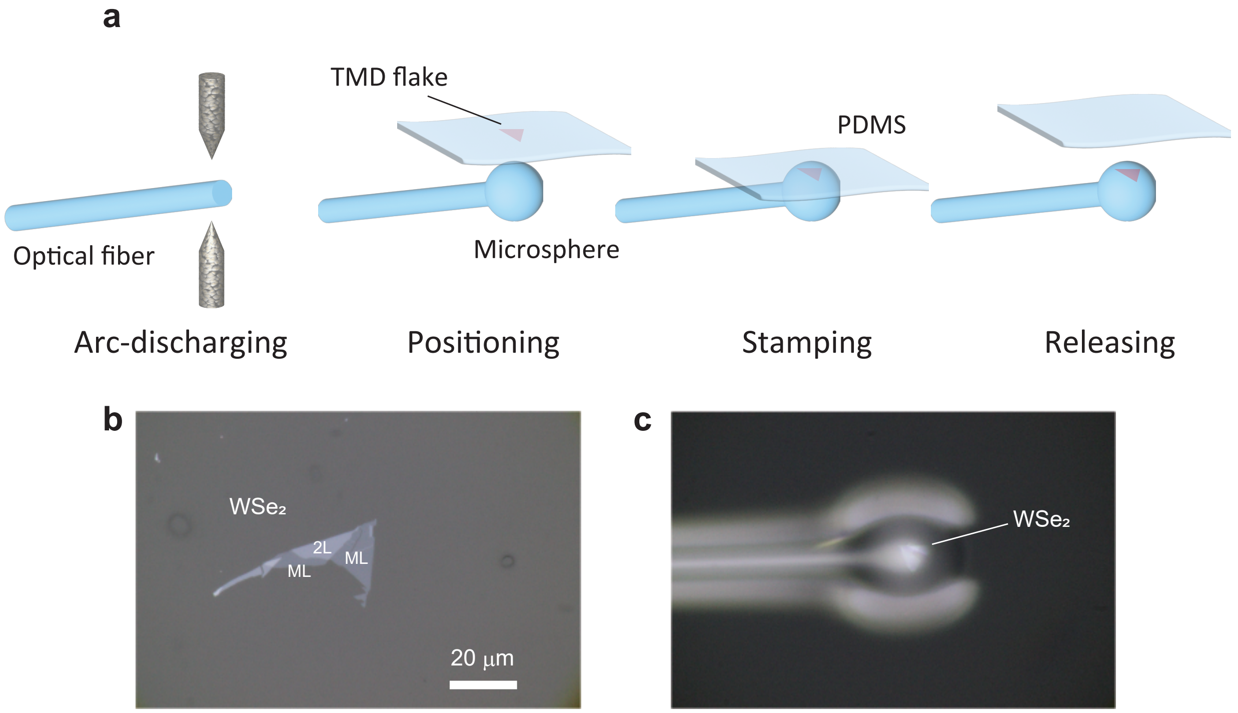


Supplementary Figure S2. Sample fabrication of 2D-material-integrated silica microspheres. (a) Fabrication process. Steps from cavity fabrication to all-dry transfer. (b, c) Microscope images of $WSe_2$ on a PDMS sheet and functionalized microsphere (image focused on the $WSe_2$ flake), respectively.

Fabrication process of 2D-material-functionalized microsphere is shown in Fig. S2(a). A device is prepared by the following steps: microsphere fabrication via arc-discharging, positioning, stamping, and releasing. Figure S2(b) and S2(c) show microscope images of the $WSe_2$ flake before and after the transfer process.

**Supplementary Note 3: SH intensity dependence on the pump polarization**

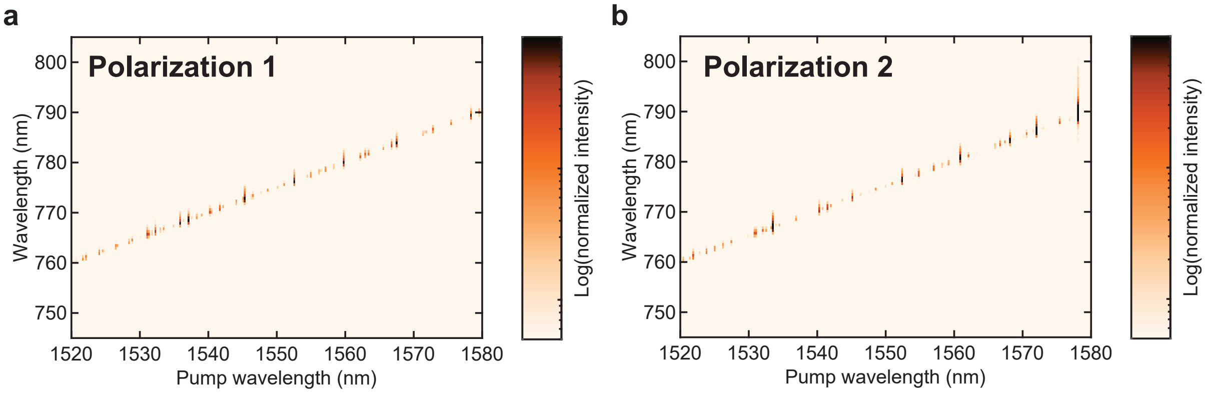


Supplementary Figure S3. Pump polarization dependence of SH light intensity. Spectral mapping of SH light intensity for two different pump polarizations (Polarization 1 and Polarization 2). The measurements are performed with a pump power of 3 mW.

The SH mapping for two different polarizations is shown in Fig. S3. We observe no significant dependence of SH intensity on the pump polarization even though the observed SH wavelengths clearly differ. The pump polarization is selected by using a fiber polarization controller before the excitation while monitoring the transmission spectrum. We note that the polarization of the SH light is not necessarily the same as the pump polarization because the SH light originated from TMD flakes exhibits a six-fold symmetric response (60° symmetry) [2] which allows coupling to either TE or TM modes.

## SUPPLEMENTARY REFERENCES

[1] H. A. Haus, *Waves and fields in optoelectronics* (Prentice Hall, 1984).

[2] Y. Li, Y. Rao, K. F. Mak, Y. You, S. Wang, C. R. Dean, and T. F. Heinz, Probing symmetry properties of few-layer $MoS_2$ and h-BN by optical second-harmonic generation, Nano Lett. **13**, 3329 (2013).
